# Supplementary material for: Collaborative Distillation for Top-N Recommendation
Source: arXiv:1911.05276 source file (2019-11-13)
Supplement: Supplementary file 1 [file appendix-table1.tex]

\begin{table*}[t!]
\begin{center}
\caption{Statistics of four benchmark datasets.}\label{tab:statistics}
%\begin{tabular}{p{1.0cm}p{1.2cm}p{1.2cm}p{2.0cm}p{1.2cm}p{4cm}p{4cm}}
\begin{tabular}{llllccc}
\toprule
Dataset & \# of users & \# of items & \# of interactions & Sparsity & min/max/avg. interactions per user & min/max/avg. interactions per item \\
\hline
AMusic & 2,831 & 13,410 & 63,054 & 99.83\% & 10/714/22.27 & 1/155/4.70 \\
ML100K & 943 & 1,682 & 100,000 & 93.70\% & 20/737/106.04 & 1/583/59.45 \\
Yelp & 9,788 & 25,373 & 489,820 & 99.80\% & 20/1024/50.04 & 1/674/19.30 \\
Gowalla & 13,149 & 14,009 & 535,650 & 99.71\% & 15/764/40.73 & 15/1743/38.24 \\
\bottomrule
\end{tabular}
\end{center}
\vskip -0.2in
\end{table*}

%\begin{table*}[t]
%\begin{center}
%\caption{Hyperparameters of our model.}\label{tab:statistics}
%\begin{tabular}{p{1.5cm}p{10cm}p{5cm}}
%\toprule
%Notation & Definition & Value \\
%\hline
%$\lambda$ & Balance the collaborative filtering loss and knowledge distillation loss in collaborative distillation & [0, 0.2, 0.4, 0.6, 0.8, 1] (default = 1) \\
%T1 & Control the scale of real-valued logit(zui) in logistic function & [0.5, 1, 2, 4] (default = 1) \\
%T2 & Control the scale of real-valued logit(zui) in logistic function & [1, 2, 4, 6, 8] (default = 1) \\
%$\delta$ &Sampling ratio of user's missing interactions for knowledge distillation & [0, 0.2, 0.4, 0.6, 0.8, 1] (default = 0.2) \\
%$\eta$ & The number of negative sampling at Caser model & [1, 3, 5, 7, 9] (default = 3) %\\
%\bottomrule
%\end{tabular}
%\end{center}
%\end{table*}
